# Supplementary material for: EasyVideoR1: Easier RL for Video Understanding
Source: arXiv:2604.16893 source file (2026-04-18)
Supplement: Supplementary file 1 [file 99_appendix.tex]

\section{Appendix}

Use the appendix for supplementary derivations, tables, prompts, or extra figures.
